# Supplementary material for: Analysis of Linux-PRNG (Pseudo Random Number Generator)
Source: arXiv:2312.03369 source file (2023-12-06)
Supplement: Supplementary file 1 [file appendix.tex]

\clearpage
\section{Appendix}
\label{app:A}
...
